# Supplementary material for: Spin-isomer conversion of water at room temperature, and quantum-rotor-induced nuclear polarization, in the water-endofullerene H$_2$O@C$_{60}$
Source: arXiv:1802.00676 ancillary file (2018-02-02)
Supplement: Supplementary file 1 [file supplementaryMaterial.pdf]

# Spin-isomer conversion of water at room temperature, and quantum-rotor-induced nuclear polarization, in the water-endofullerene $H_2O@C_{60}$: Supplemental material

Benno Meier, Karel Kouřil, Christian Bengs, Hana Kouřilová, Timothy J. Barker, Stuart J. Elliott, Shamim Alom, Richard J. Whitby, and Malcolm H. Levitt

*School of Chemistry, University of Southampton, Southampton, SO17 1BJ, United Kingdom*

(Dated: January 31, 2018)

## CAPACITANCE APPARATUS

The probe used to measure the capacitances of $H_2O@C_{60}$, $H_2{}^{16}O@C_{60}$, and $H_2{}^{17}O@C_{60}$ is shown in Fig. S2. A solid steel rod (Wellington Tube Supplies, UK) of length 130 mm and diameter 1/16" forms the inner electrode. The outer electrode (Wellington Tube Supplies) is a steel tube with outer diameter 3/16" and wall thickness 0.55 mm. A brass disk is brazed to the outer electrode to facilitate easy soft-soldering of a copper wire. A second copper wire is brazed to the inner electrode. After loading the sample with a syringe the inner electrode is placed into the capacitor, and the copper wire is soldered to a pad on a printed-circuit board that hosts SMA connectors for each capacitor. The copper wire of the outer electrode is soldered to another circuit board at the bottom of the probe. RG-147 cable (RS Components, UK) is used to connect the circuit-board to feed-throughs on a KF-50 cross (Kurt J. Lesker, UK) at the top of the probe. The cables run on the inside and outside of a glass-fibre enforced plastic tube (Shannonvale Fibre Tubes, Ireland). A cernox temperature sensor is attached to the probe with PTFE tape. The capacitances are measured using an AD7746 capacitance to digital converter (Analog Devices, US) as detailed in the Supplementary Information of Ref. [1]. A measurement of the capacitances of the empty capacitors yielded 6.55, 6.80, and 6.64 pF for the capacitors that were subsequently filled with $H_2O@C_{60}$, $H_2{}^{16}O@C_{60}$ and $H_2{}^{17}O@C_{60}$ in ODCB, respectively.

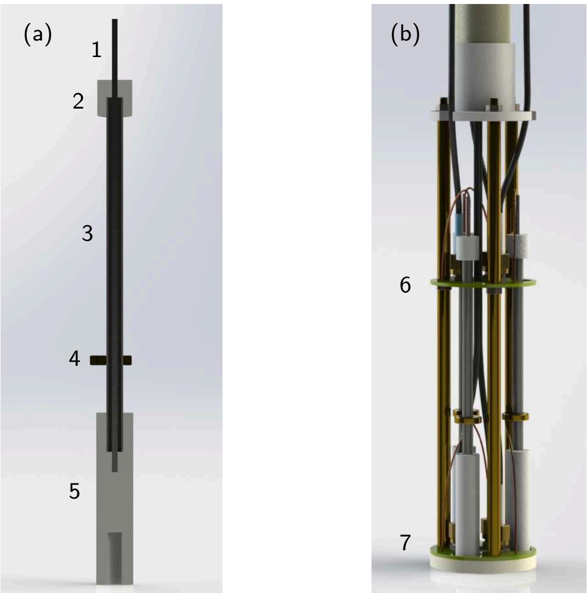


FIG. S1. Capacitance Setup. (a) Cross-section of a single capacitor. The inner electrode (1, steel) is pushed through a lid (2, PEEK) and centered by a drilled hole in the bottom support (5, PTFE). The outer electrode (3, steel) is also pushed into the bottom support to form a tight seal. A brass disk (4) is brazed onto the outer electrode. (b) (b) The capacitance probe comprises three capacitors as shown in (a). One copper wire is soldered to the brass disk, a second copper wire is brazed to the inner electrode. The copper wires of the inner electrode are soldered to corresponding pads on two printed circuit boards (PCB) (6, 7) that each host three SMA connectors.

## CAPACITANCE DATA PROCESSING

Experimental data are shown in Fig. S2. Panel (a) shows a measurement of the temperature during 10 h before, and 28 h after the temperature jump. Panel (b) shows the same data, but re-scaled to show the small fluctuations of 5.05$\pm$0.03 K. Panels (c-e) show the raw capacitance data as measured on the capacitors for $H_2O@C_{60}$, $H_2{}^{16}O@C_{60}$, and $H_2{}^{17}O@C_{60}$, respectively. The corrected data, shown in panels (f) and (g), are obtained by dividing the raw values by those of the $H_2O@C_{60}$ capacitor for each point. Data prior to the temperature drop are multiplied with the mean value of the $H_2O@C_{60}$ capacitor prior to the temperature drop, data after the temperature drop are multiplied with the mean value of the $H_2O@C_{60}$ capacitor after the temperature drop. The black curves in panels (f,g) show bandwidth-reduced versions of the respective data, that are obtained using local linear regression with a “tri-cube” kernel

$$k(x_p;x) = \begin{cases} \left(1-|(x_p-x)/h|^3\right)^3 & \text{for } |\mathrm{x_p}-\mathrm{x}| < \mathrm{h} \\ 0 & \text{otherwise} \end{cases}$$

with a width $h = 5\,\mathrm{min}$ as detailed in Ref. [2].

## CAPACITANCE DATA MODELLING

The bulk polarizability of a sample $\mathcal{P}(\epsilon)$ is a function of the dielectric constant $\epsilon$, and may be calculated using the Clausius-Mossotti equation:

$$\mathcal{P}(\epsilon) = 3\epsilon_0 \frac{\epsilon - 1}{\epsilon + 2}. \tag{1}$$

Here, we are interested only in changes of the electrical polarizability, which occur as the dielectric constant changes. We define

$$\Delta\mathcal{P}(t) = \mathcal{P}(\epsilon(t)) - \mathcal{P}(\epsilon(-1\,\mathrm{h})), \tag{2}$$

that is, changes are referenced to the value of the polarizability 1 h before the temperature drop. Using the known volume density, it is possible to calculate the change in average polarizability volume $\Delta\alpha\prime = (\Delta P/N)/(4\pi\epsilon_0)$ of $H_2{}^{16}O@C_{60}$ and $H_2{}^{17}O@C_{60}$.

Corresponding data are shown in Fig. S3, along with fits to an exponential model (left column, a-d), and a second order model (right column, e-h). The fit residues for exponential and second order models are shown in panels (b) and (d) for the exponential model, and in panels (f) and (h) for the second order model. The residue in panel (d) reveals correlated deviations between fit and data, that are not present with the second order fit (residue shown in panel (h)). Therefore the $H_2{}^{17}O@C_{60}$ data are more accurately described using a second order model.

The exponential model takes the form

$$F(t) = A\exp(-t/\tau) + B. \tag{3}$$

The second order model takes the form

$$G(t) = \frac{C}{1+kt} + D. \tag{4}$$

Obtained fit values for both models for both $H_2{}^{16}O@C_{60}$ and $H_2{}^{17}O@C_{60}$ are given in Tab. S1.

| | A (Å$^3$) | B (Å$^3$) | $\tau$ (h) | C (Å$^3$) | D (Å$^3$) | $k$ (h$^{-1}$) |
|---|---|---|---|---|---|---|
| $H_2{}^{16}O@C_{60}$ | 1.116(4) | 8.800(9) | 15.2(3) | 1.63(1) | 8.30(2) | 0.051 (1) |
| $H_2{}^{17}O@C_{60}$ | 1.029(9) | 11.518(2) | 2.88(4) | 1.31(1) | 11.414(2) | 0.67(1) |

TABLE S1. Fit parameters obtained for the *ortho*-to-*para* conversion of $H_2O@C_{60}$ in ODCB . Columns 2-4 give estimates for an exponential model, columns 5-7 give estimates for a second order model. The values in parentheses give the uncertainty in the last digit as obtained from the Levenberg-Marquardt non-linear least squares algorithm.

## ORTHO/PARA-CONVERSION IN SOLID SAMPLES

The same analysis as above may also be applied to a measurement of the capacitance of solid pellets of $H_2{}^{16}O@C_{60}$ and $H_2{}^{17}O@C_{60}$, using the same apparatus and methodology as described in Ref. [1]. As detailed in the supporting information of Ref. [1], it is permissible to extract the kinetic parameters directly from the measured capacitance data, since changes in the dielectric constant are small. The corresponding data are shown in Fig. S4, along with fits according to equations (3) and (4). The conversion proceeds faster in $H_2{}^{17}O@C_{60}$, and the second order model yields better agreement with the experimental data. Fit results are given in Tab. S2.

| | A (pF) | B (pF) | $\tau$ (h) | C (pF) | D (pF) | $k$ (h$^{-1}$) |
|---|---|---|---|---|---|---|
| $H_2{}^{16}O@C_{60}$ | 0.409(2) | 14.552(2) | 3.83(6) | 0.538(1) | 14.454(1) | 0.309(3) |
| $H_2{}^{17}O@C_{60}$ | 0.254(2) | 12.935(6) | 2.05(3) | 0.3262(3) | 12.9002(1) | 0.823(2) |

TABLE S2. Fit parameters obtained for the *ortho*-to-*para* conversion of solid $H_2O@C_{60}$ pellets . Columns 2-4 give estimates for an exponential model, columns 5-7 give estimates for a second order model. The values in parentheses give the uncertainty in the last digit as obtained from the Levenberg-Marquardt non-linear least squares algorithm.


[1] B. Meier, S. Mamone, M. Concistrè, J. Alonso-Valdesueiro, A. Krachmalnicoff, R. J. Whitby, and M. H. Levitt, Nature Communications **6**, 8112 (2015).

[2] P. K. Janert, *Data Analysis with Open Source Tools* (O'Reilly, 2010).

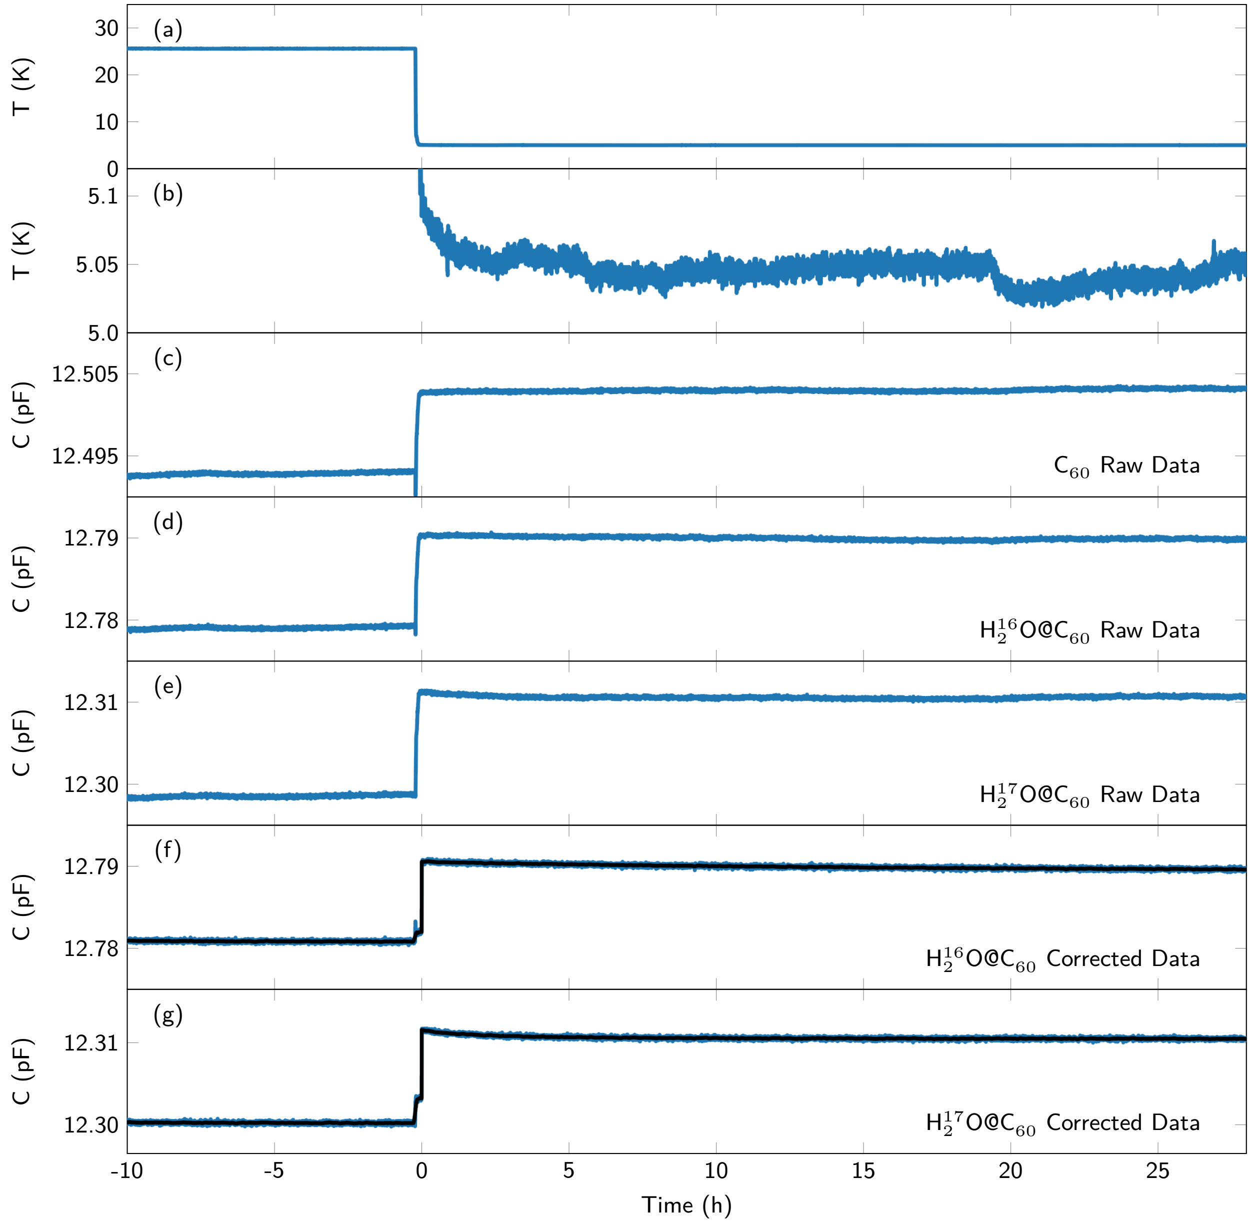


FIG. S2. Capacitance data. (a) Temperature profile. (b) The same data as in (a), but re-scaled to show temperature fluctuations. (c-e) Raw capacitance data of the capacitors filled with ODCB containing (i) $C_{60}$, (ii) $H_2{}^{16}O@C_{60}$, and (iii) $H_2{}^{17}O@C_{60}$, respectively. (f-g) Corrected capacitance data of $H_2{}^{16}O@C_{60}$ and $H_2{}^{17}O@C_{60}$, respectively. The black curves show bandwidth-reduced versions of the respective data.

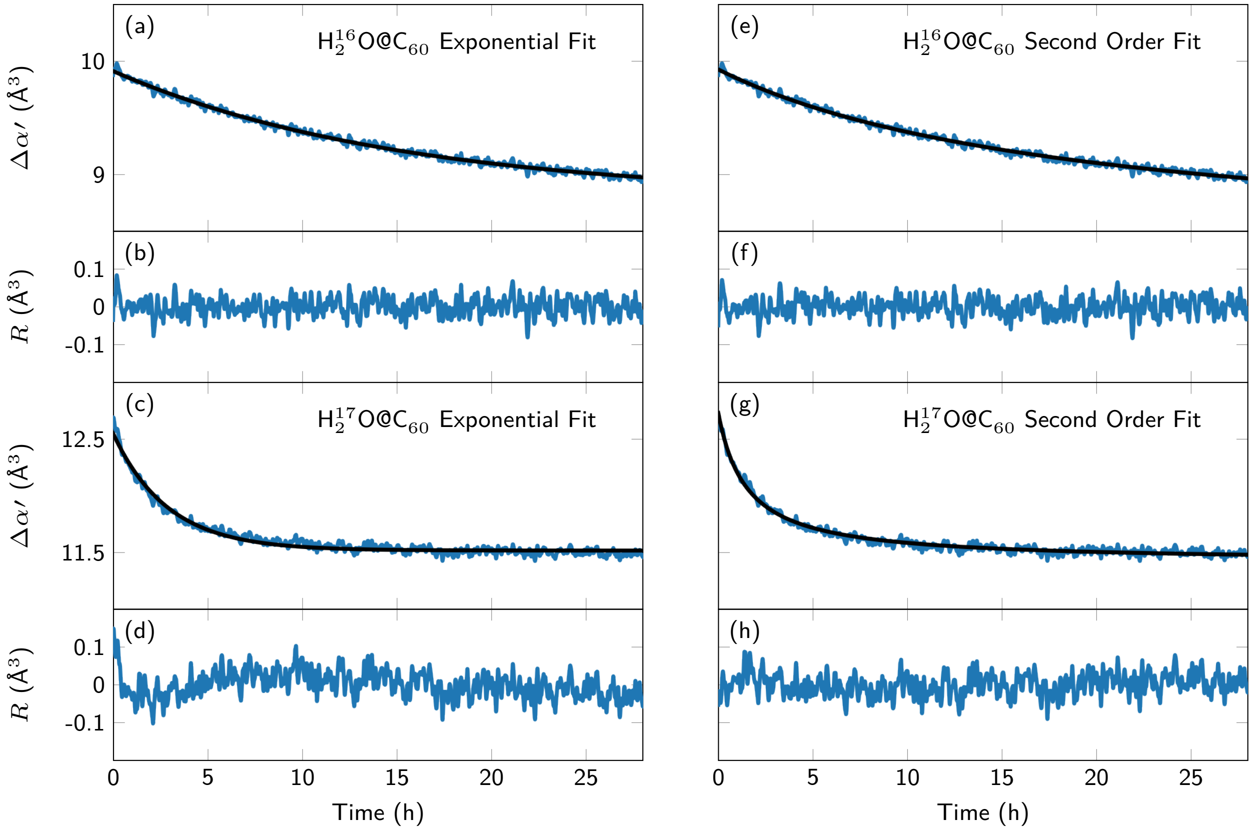


FIG. S3. Change in polarizability volume $\Delta\alpha'$ for $H_2{}^{16}O@C_{60}$ and $H_2{}^{17}O@C_{60}$ in ODCB modelled using an exponential decay (left column) or second order kinetics (right column). (a) Change in polarizability volume relative to the measured volume prior to the temperature drop for $H_2{}^{16}O@C_{60}$ (blue curve), along with an exponential fit (black curve). (b) Difference between data and fit. (c,d) The same data as in (a,b) but for $H_2{}^{17}O@C_{60}$. The residue in (d) reveals correlated deviations between the exponential fit and the data for $H_2{}^{17}O@C_{60}$ (e-h) The same data as in (a-d), but with second order models and corresponding residues. The $H_2{}^{17}O@C_{60}$ data are accurately described by second order kinetics.

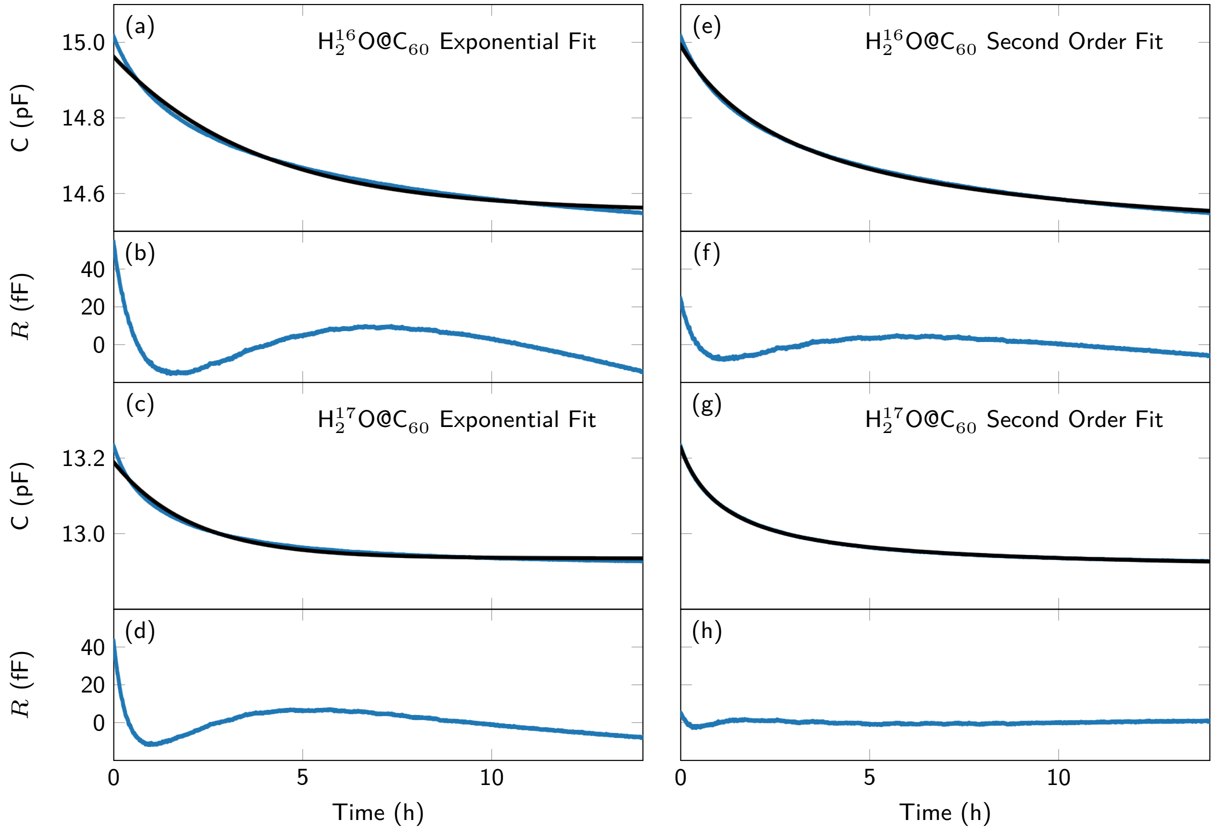


FIG. S4. Capacitance measurement of solid $H_2{}^{16}O@C_{60}$ and $H_2{}^{17}O@C_{60}$ pellets, modelled using an exponential decay (left column) or second order kinetics (right column). (a) Capacitance of a plate capacitor filled with $H_2{}^{16}O@C_{60}$ (blue curve) following a temperature drop from 30 to 5 Kelvin, along with an exponential fit (black curve). (b) Difference between data and fit. (c,d) The same data as in (a,b) but for $H_2{}^{17}O@C_{60}$. The same data as in (a-d), but with second order models and corresponding residues. The second order model gives better agreement for both samples, but correlated deviations are seen in particular for $^{16}O$.
